# Supplementary material for: MultiON: Benchmarking Semantic Map Memory using Multi-Object Navigation
Source: arXiv:2012.03912 source file (2020-12-07)
Supplement: Supplementary file 1 [file neurips_2020_additional_experiments.tex]

\documentclass{article}
\PassOptionsToPackage{numbers, compress}{natbib}
\usepackage{neurips_2020}

\input{macros}

\title{Multi-ON: Benchmarking Semantic Map Memory using Multi-Object Navigation\\Additional Experiments}
\usepackage{rotating}

\author{%
  Saim Wani$^{1}$\qquad
  Shivansh Patel$^{1}$\qquad
  Unnat Jain$^{2}$\qquad
  Angel X. Chang$^{3}$\qquad
  Manolis Savva$^{3}$\\
  $^{1}$IIT Kanpur\qquad$^{2}$UIUC$^{3}$SFU\\
}

\begin{document}

\maketitle

\section{Additional Material}

\SW{
\subsection{Visualizing learnt models through Grad-CAM}
To understand what parts what parts of the map or the RGBD frame the model is attending to while choosing an action, we visualize the gradient-weighted Class Activation Maps (Grad-CAM)~\cite{selvaraju2016grad} of the two. For doing so, we use the gradients of the sampled action (likely to be the action with a higher score) flowing into the final constitutional layer. We do this for both the CNNs: the one  processing the Map and the one processing the RGBD frame and produce a localization map highlighting the important regions in the map for the predicted action. 

\textit{There doesn't seem to be anything interesting in the visualizations, what frame should I put here? The only time something slightly remarkable appears in the visualizations is when an object is in view and the heatmap is focused on it.}
}

\end{document}
